# Supplementary material for: Who Walks With You Matters: Perceiving Social Interactions with Groups for Pedestrian Trajectory Prediction
Source: arXiv:2412.02395 source file (2024-12-03)
Supplement: Supplementary file 2 [file appendix_f2_contribution_ratio.tex]

%%%%%%%%%%%%%%%%%%%%%%%
%% Author: Ziqian Zou
%% Date: 2024-11-19 10:25:56
%% LastEditors: Ziqian Zou
%% LastEditTime: 2024-11-22 10:38:10
%% Description: file content
%% Github: https://github.com/LivepoolQ
%% Copyright 2024 Ziqian Zou, All Rights Reserved.
%%%%%%%%%%%%%%%%%%%%%%%
\documentclass[../paper.tex]{subfiles}

\begin{document}

\begin{figure}[t]
    \centering
    \includegraphics[width=1.0\linewidth]{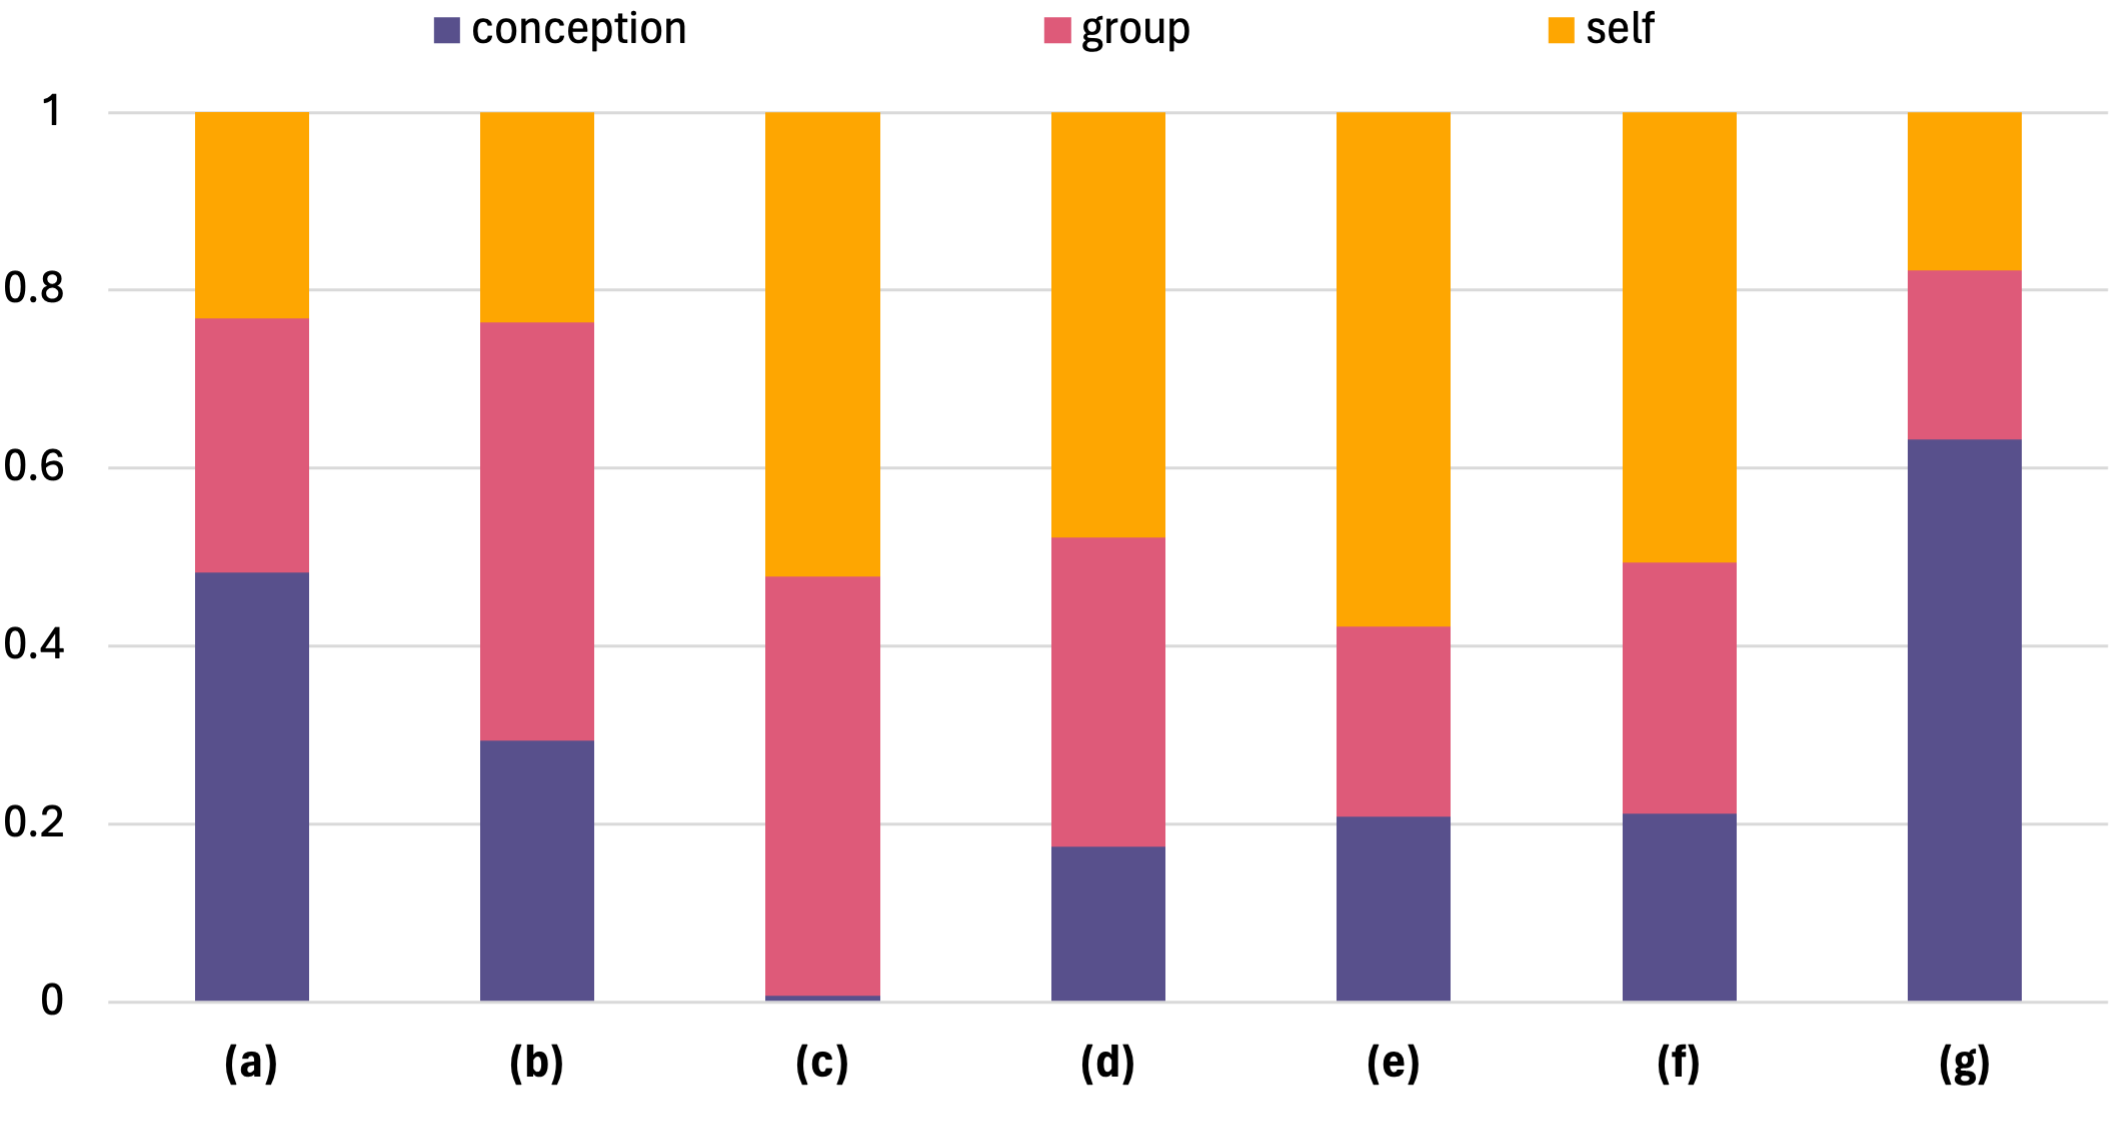}
    \caption{
        Contribution ratio of the \textcolor[RGB]{88,80,141}{\textbf{Conception}} feature, the \textcolor[RGB]{222,90,79}{\textbf{Group}} feature and the \textcolor[RGB]{255,166,00}{\textbf{Self}} feature in the form of bar charts.
        Each bar corresponds to Fig. 5 in the main manuscript.
    }
    \label{fig_contribution_ratio}
\end{figure}

\end{document}
